# Supplementary material for: MoTCoder: Elevating Large Language Models with Modular of Thought for Challenging Programming Tasks
Source: arXiv:2312.15960 source file (2025-03-30)
Supplement: Supplementary file 1 [file appendix.tex]

\newpage
\appendix
\iffalse
\subsection{LeetCode Examples}
For given input problems, we provided samples generated by WizardCoder~\cite{wizardcoder} and MoTCoder. Upon manually examination, we noted that MoTCoder consistently produces superior programs, characterized by effective modularization and explanations through function docstrings. we provided samples generated by WizardCoder~\cite{wizardcoder} and MoTCoder and the output codes are examined by LeetCode website. 

\begin{figure*}[p]
\centering
% \vspace{-2mm}
\includegraphics[width=0.95\linewidth, trim=10 55 230 3, clip]{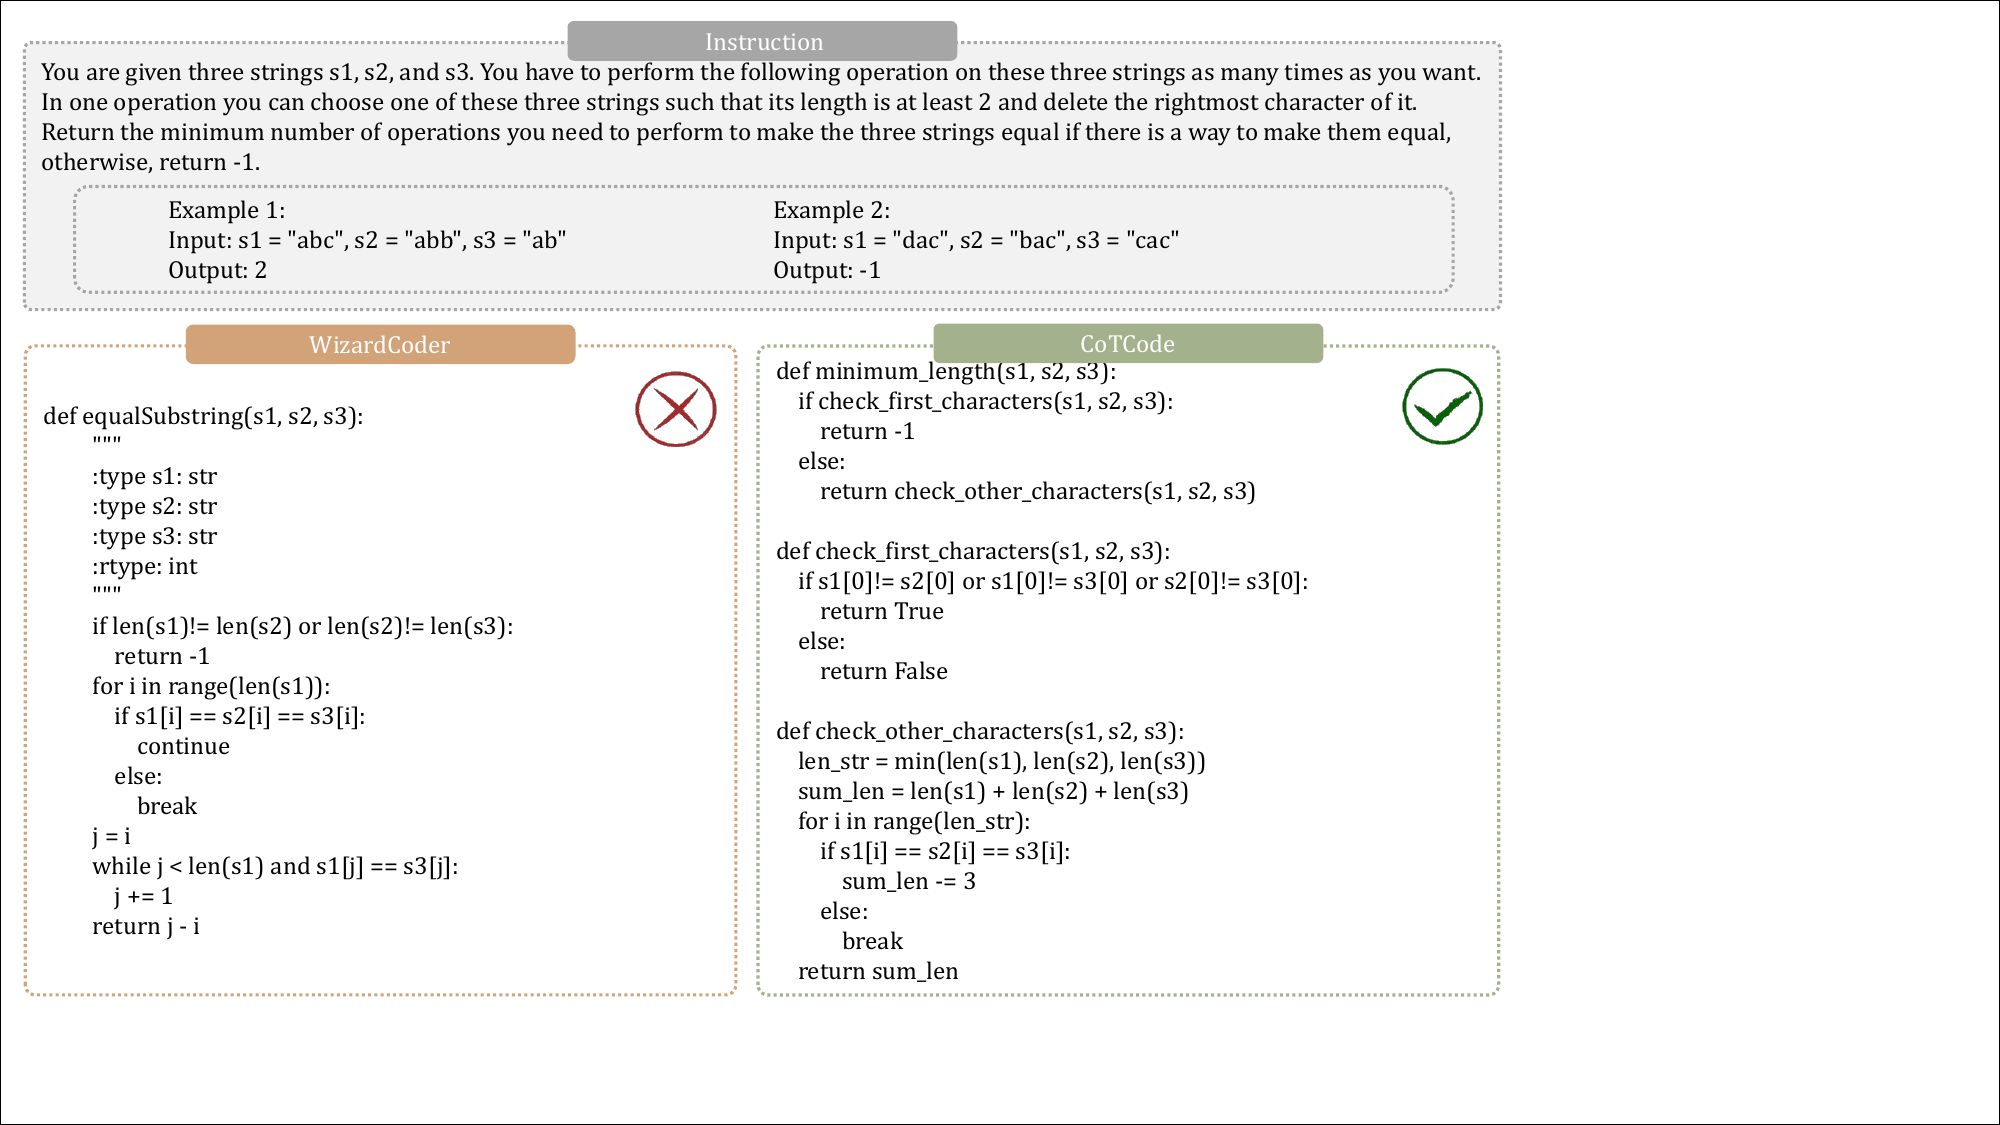}
\includegraphics[width=0.95\linewidth, trim=10 10 230 3, clip]{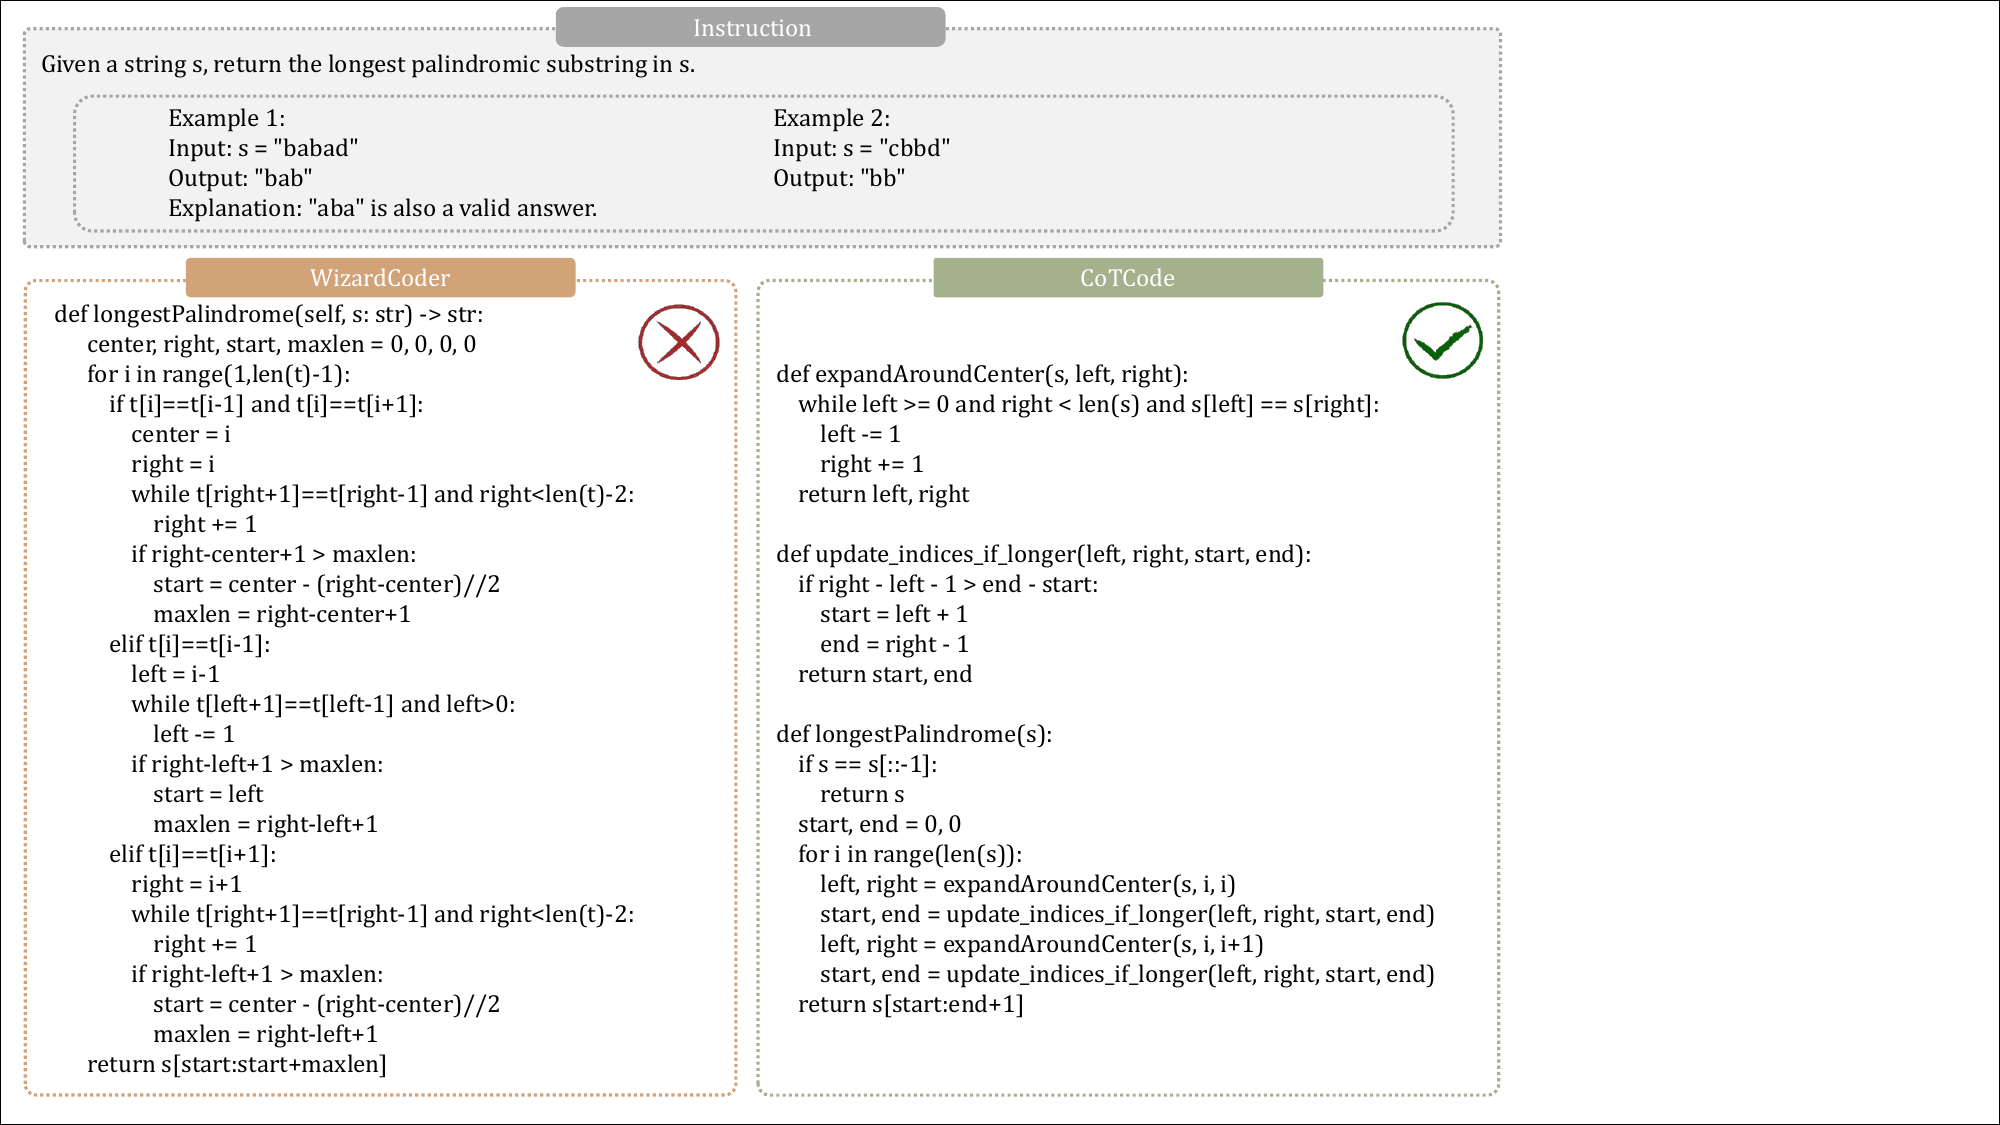}
% \vspace{-3mm}
\caption{Examples of problems and generation samples generated by WizardCoder~\cite{wizardcoder} and MoTCoder.}
\label{fig:examples}
\end{figure*}
\fi

%%%%%%%%%%%%%%%%%%%%%%%%%%%%%%%%%%%%%%%%%%%%%%%%%%
%%%%% APPs EXamples
%%%%%%%%%%%%%%%%%%%%%%%%%%%%%%%%%%%%%%%%%%%%%%%%%%
% \subsection{APPs Examples}
\section{Examples}
\label{sec:examples}
For given input problems, we provided submodules and final code solution examples for problems from APPs test dataset. 
\subsubsection{APPs Example 1}
\begin{table}[t]
    \centering
    \color{blue}
    \begin{tabular}{p{\linewidth}}
        \textbf{Original Solution} \\
\begin{lstlisting}
for _ in range(int(input())):
    s = input()

    ones = []
    cnt = 0
    for i in s:
        if i == '1':
            cnt += 1
        else:
            if cnt != 0:
                ones.append(cnt)
                cnt = 0
    if cnt != 0:
        ones.append(cnt)

    ones.sort(reverse=True)
    print(sum(ones[::2]))
\end{lstlisting} \\
        \textbf{MoT Solution} \\
\begin{lstlisting}
def calculate_alice_score(binary_string):
    """
    This function calculates Alice's score by extracting continuous segments of '1's, sorting them in descending order, and summing up the counts that Alice would pick.
    """
    ones_groups = []
    current_count = 0

    # Extract groups of consecutive '1's
    for char in binary_string:
        if char == '1':
            current_count += 1
        else:
            if current_count > 0:
                ones_groups.append(current_count)
                current_count = 0

    # Append the last segment if it ends with '1's
    if current_count > 0:
        ones_groups.append(current_count)

    # Sort segments in descending order to maximize Alice's score
    ones_groups.sort(reverse=True)

    # Alice selects the first, third, fifth ... largest groups
    return sum(ones_groups[::2])

# Process multiple test cases
test_cases = int(input())

for _ in range(test_cases):
    binary_string = input().strip()
    print(calculate_alice_score(binary_string))
\end{lstlisting} \\
    \end{tabular}
    \caption{Comparison of Original and MoT Solutions for Binary String Processing.}
    \label{tab:data_example}
\end{table} 

\subsubsection{APPs Example 2}
\input{append_tables/apps_example_2}
